# Supplementary material for: Q-Pensieve: Boosting Sample Efficiency of Multi-Objective RL Through Memory Sharing of Q-Snapshots
Source: arXiv:2212.03117 source file (2024-07-25)
Supplement: Supplementary file 1 [file appendix2.tex]

\section{Additional Experiments}

\section{Mixture-of-Expert Critic}
 Predicting $Q$ for different policies is like a multi-task problem. The multi-task model learns the communication and the difference in preferences to avoid learning the different tasks individually, which can reduce loss and improve learning efficiency. Besides, We revise the model proposed by \cite{10.1145/3219819.3220007} to \ref{fig:MMOE Model}. It uses weight gate to tunning the weight of different experts to handle infinite tasks. 
 We first formulate the output soft $Q(s,a;\blambda)$. It would be
 \begin{align*}
      Q(s,a;\blambda) = h(F(s,a;\blambda))\\
            \end{align*} 
      where
       \begin{align*}F(s,a;\blambda)=\sum_{i=0}^{n} g(\blambda)f_{i}(s,a) 
 \end{align*} 
 
 $h$ is tower network, $f_i(s,a),i=1,...,n$ are n expert networks that extract the feature from state action pairs and $g(\blambda)$ is the weight gating network that gives weight for n experts.
 The gating networks are simply linear transformations of the input with a softmax layer:
 \begin{align*}
     g(\blambda)=softmax(W(\blambda))
 \end{align*}
 where $W_{g} \in \mathbb{R} ^{n \times d}$ is a trainable matrix, $d$ is the feature dimension.

\subsubsection{Does MMoE critic enhance the performance?}
We may be curious about the improvement using MMoE model to construct critics. We compare
MMoE critic and normal critic, constructed by a simple layer neural network with the loss between Monte-Carlo estimation from policy and critic output and total reward and set $N_\omega = 4$ and no $Q$ buffer. We show the results in Table \ref{tab:MMOE result}. What's more, from Figure \ref{fig:MMOEHV}, we find that MMoE sacrifices some performance in some situations, especially in the preferences that focus on control cost.
Looking at \ref{fig:MMOEhv_hc}, we find that the solution set of HalfCheetah from MMoE is scattered mainly in two groups. It causes that MMoE has a bad performance from hypervolume, but it represents a good performance in our goal, total reward (see appendix) in most preference.
We also demonstrate the difference of 100 preferences in Figure \ref{fig:MMOEEPD}.

\begin{table*}[!htb]
    \centering
    \caption{Comparison with MMoE critic and Normal critic using three metric. The EPD is calculated by comparing to Standard MOSAC. And we use different reference point from Table \ref{tab:expResult} to calculate in hopper due to the larger control cost.}
    \label{tab:MMOE result}
    \begin{tabular}{l c c c }
         \hline Environments & Metrics & \textbf{Standard MOSAC} & \textbf{MMoE MOSAC} \\
         \hline
         \hline
          & HV($\times 10^6$) & \textbf{33.05} & 30.87\\
         \cline{2-4}
         HalfCheetah & UT &  4973.31& \textbf{5463.10}\\
         \cline{2-4}
          & EPD &   - &  \textbf{0.74}\\
         \hline
          & HV($\times 10^5$)& 11.03 & \textbf{15.41}\\
         \cline{2-4}
         Hopper & UT & 417.29 & \textbf{561.32} \\
         \cline{2-4}
          & EPD &  - & \textbf{0.64}\\
         
         \hline
    \end{tabular}
\end{table*}

% \begin{figure*}[!tb]
% \centering
% $\begin{array}{c c c}
%     \multicolumn{1}{l}{\mbox{\bf }} & \multicolumn{1}{l}{\mbox{\bf }} \\ 
%     \hspace{-0mm} \scalebox{0.5}{\includegraphics[width=\textwidth]{./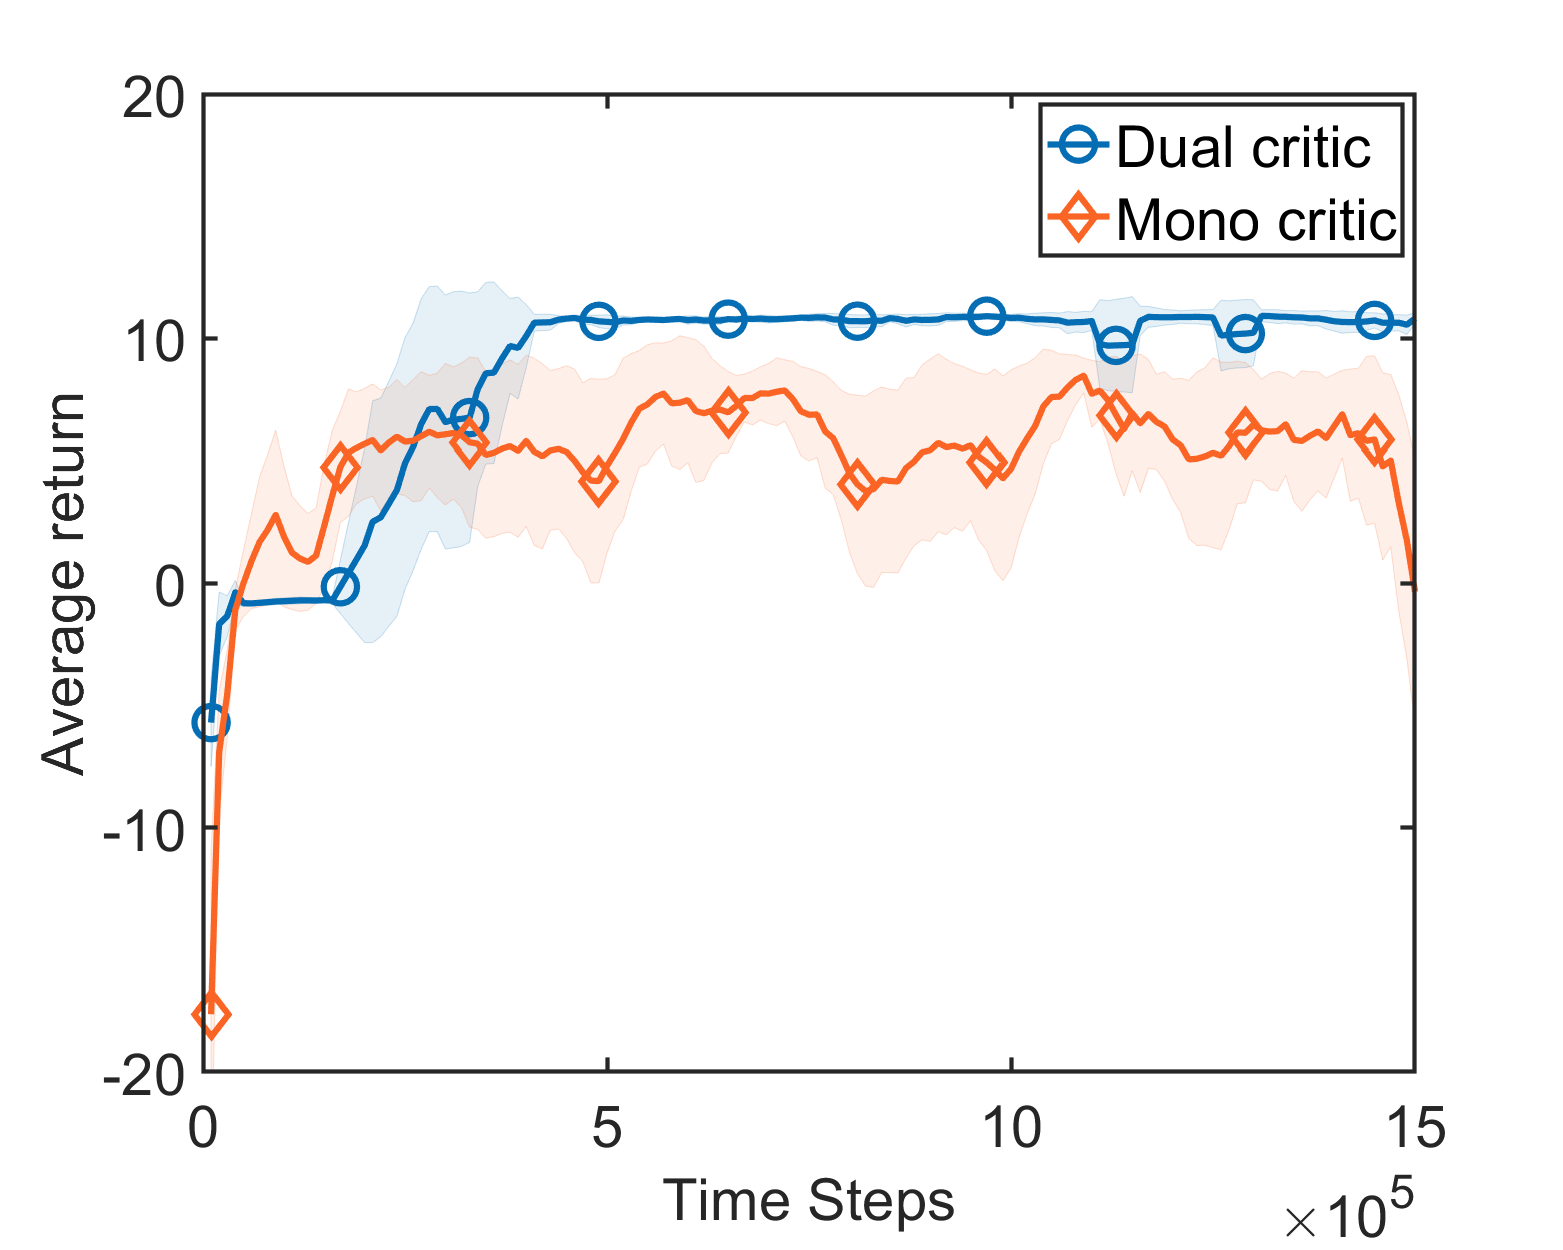}} \label{fig:Mono_vs_dual_reward19}

%     &\hspace{-5mm} \scalebox{0.5}{\includegraphics[width=\textwidth]{./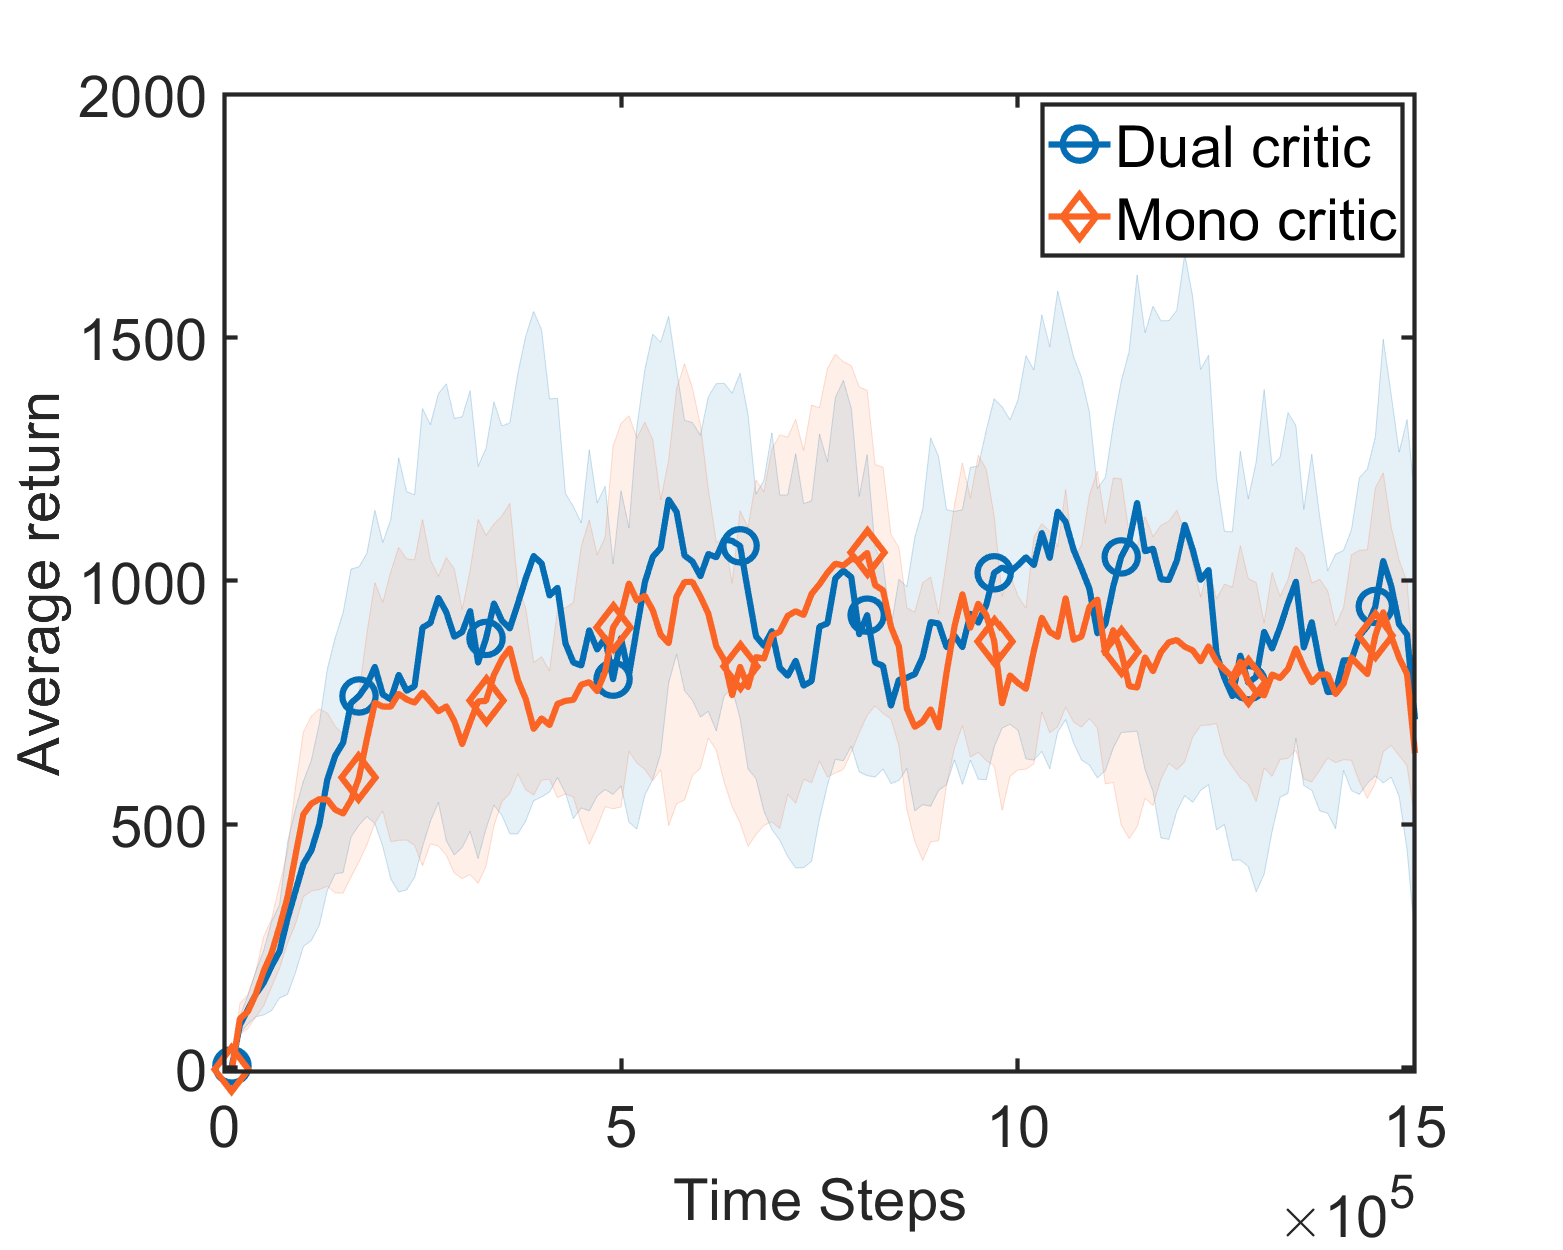}}  \label{fig:Mono_vs_dual_reward91}\\
%     \mbox{\hspace{-0mm}\small (a) $\blambda = [0.1, 0.9]$} & \hspace{-2mm} \mbox{\small (b) $\blambda = [0.9, 0.1]$}  \\
%     \multicolumn{1}{l}{\mbox{\bf }} & \multicolumn{1}{l}{\mbox{\bf }}  \label{fig:Mono_vs_dual_reward19}
% \end{array}$
% \caption{Average return in Hopper: Average return is inner product of distinct reward vectors and the corresponding preference over 5 seeds.}
% \label{fig:Mono_vs_dual_reward}
% \end{figure*}

% \begin{figure*}[!tb]
% \centering
% $\begin{array}{c c c}
%     \multicolumn{1}{l}{\mbox{\bf }} & \multicolumn{1}{l}{\mbox{\bf }} \\ 
%     \hspace{-0mm} \scalebox{0.5}{\includegraphics[width=\textwidth]{./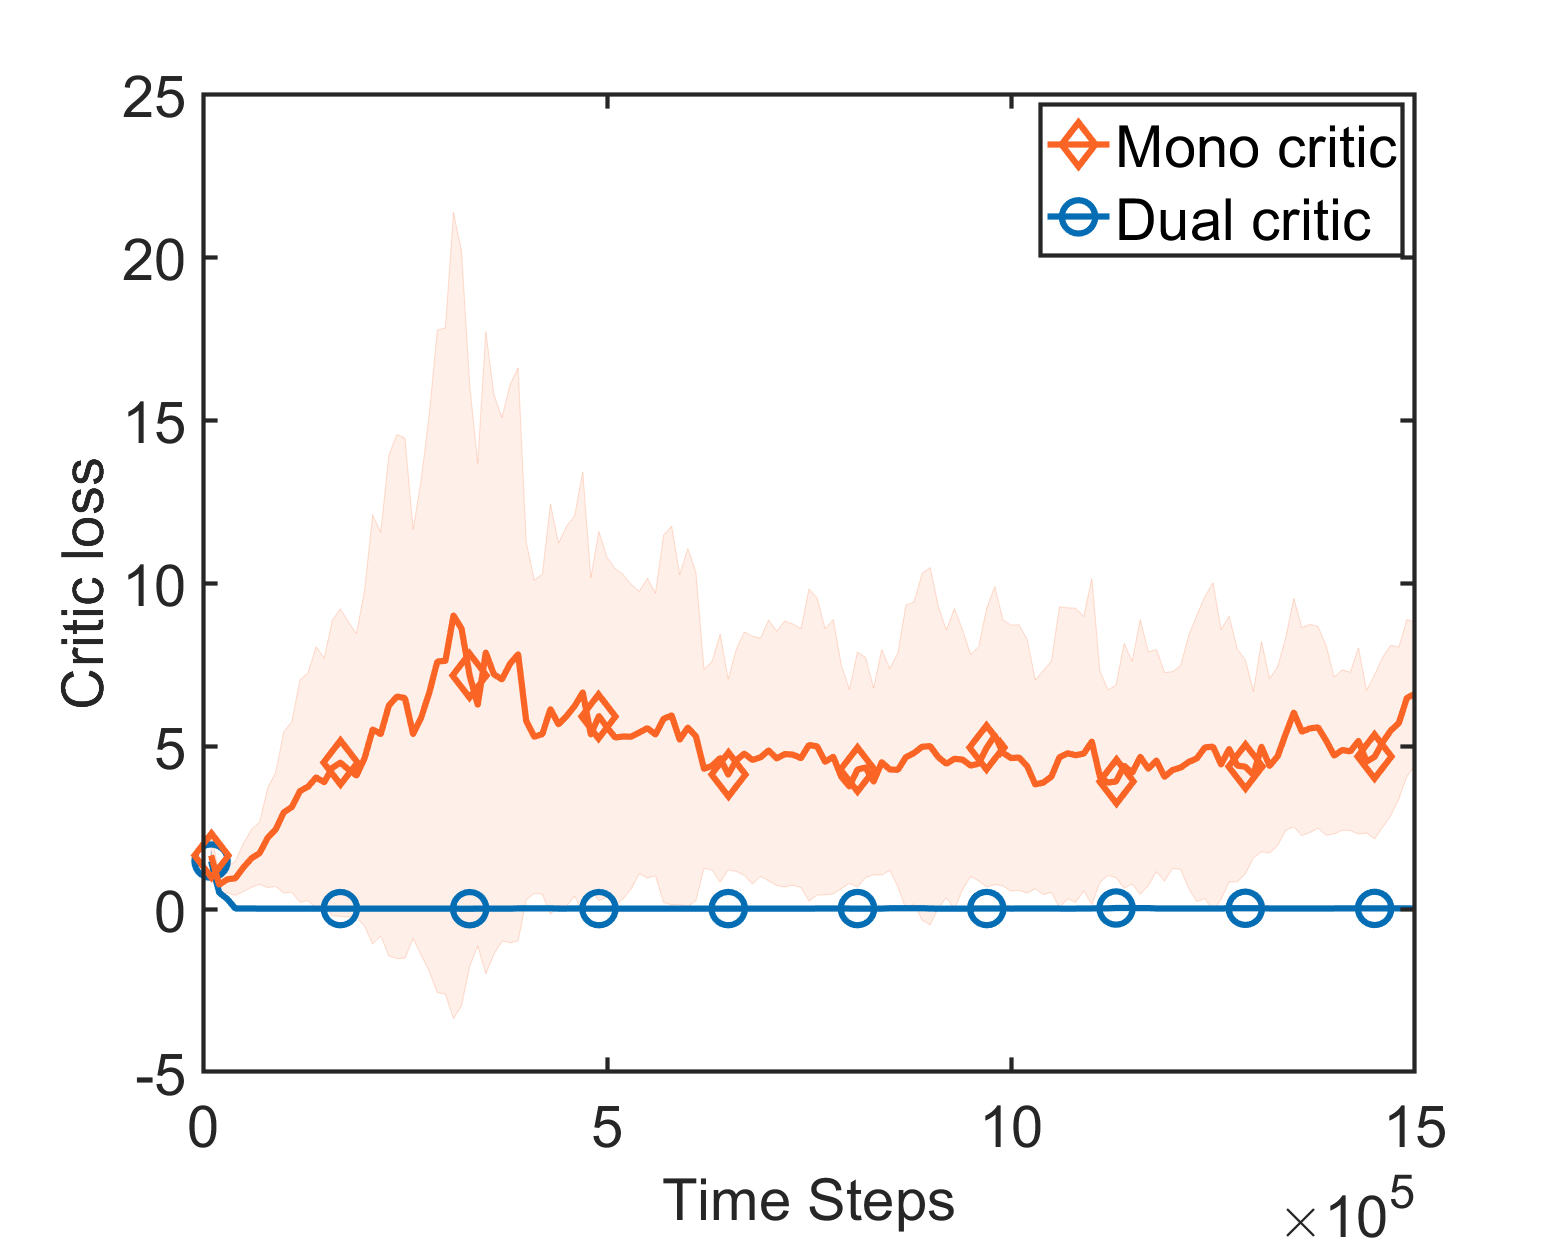}} \label{fig:Mono_vs_dual_loss19}

%     &\hspace{-5mm} \scalebox{0.5}{\includegraphics[width=\textwidth]{./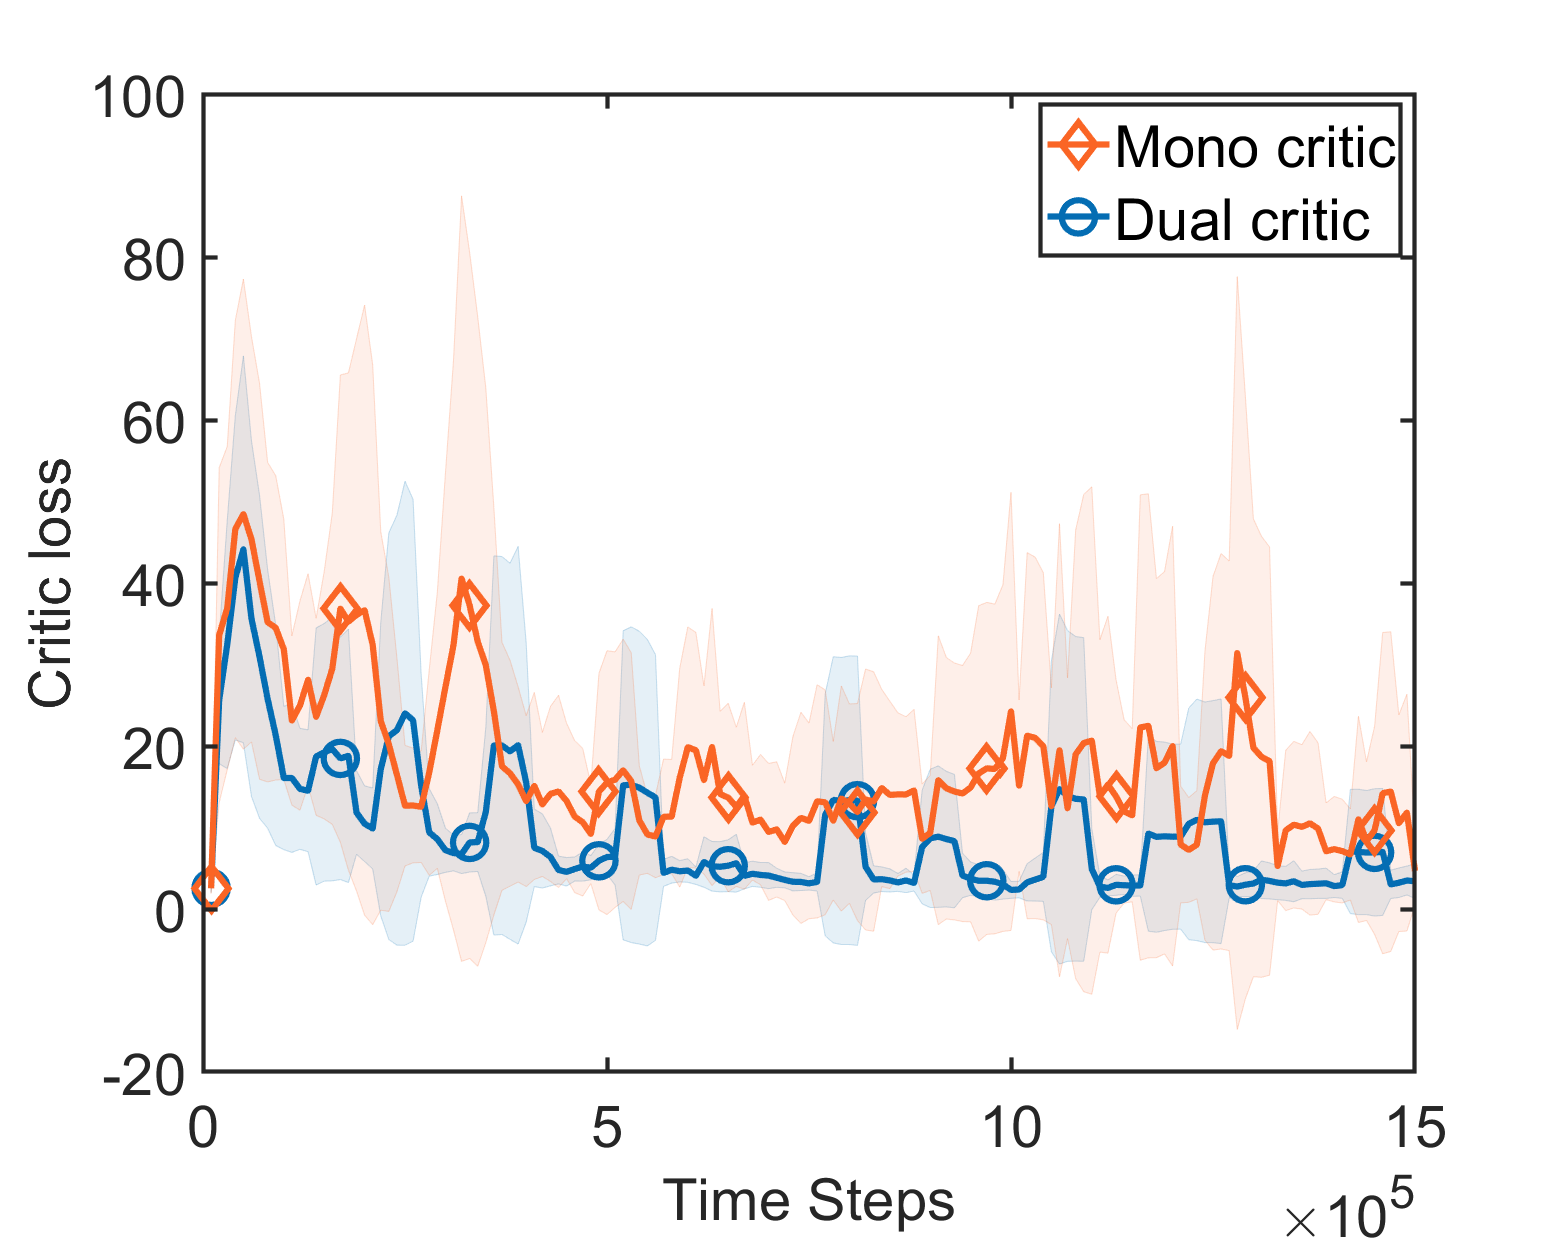}}  \label{fig:Mono_vs_dual_loss91}\\
%     \mbox{\hspace{-0mm}\small (a) $\blambda = [0.1, 0.9]$} & \hspace{-2mm} \mbox{\small (b) $\blambda = [0.9, 0.1]$}  \\
% \end{array}$
% \caption{Critic loss in Hopper: Critic loss is MSE loss of critics.}
% \label{fig:Mono_vs_dual_loss}
% \end{figure*}

\begin{figure*}[!tb]
\centering
$\begin{array}{c c c}
    \multicolumn{1}{l}{\mbox{\bf }} & \multicolumn{1}{l}{\mbox{\bf }} \\ 
    \hspace{-0mm} \scalebox{0.5}{\includegraphics[width=\textwidth]{./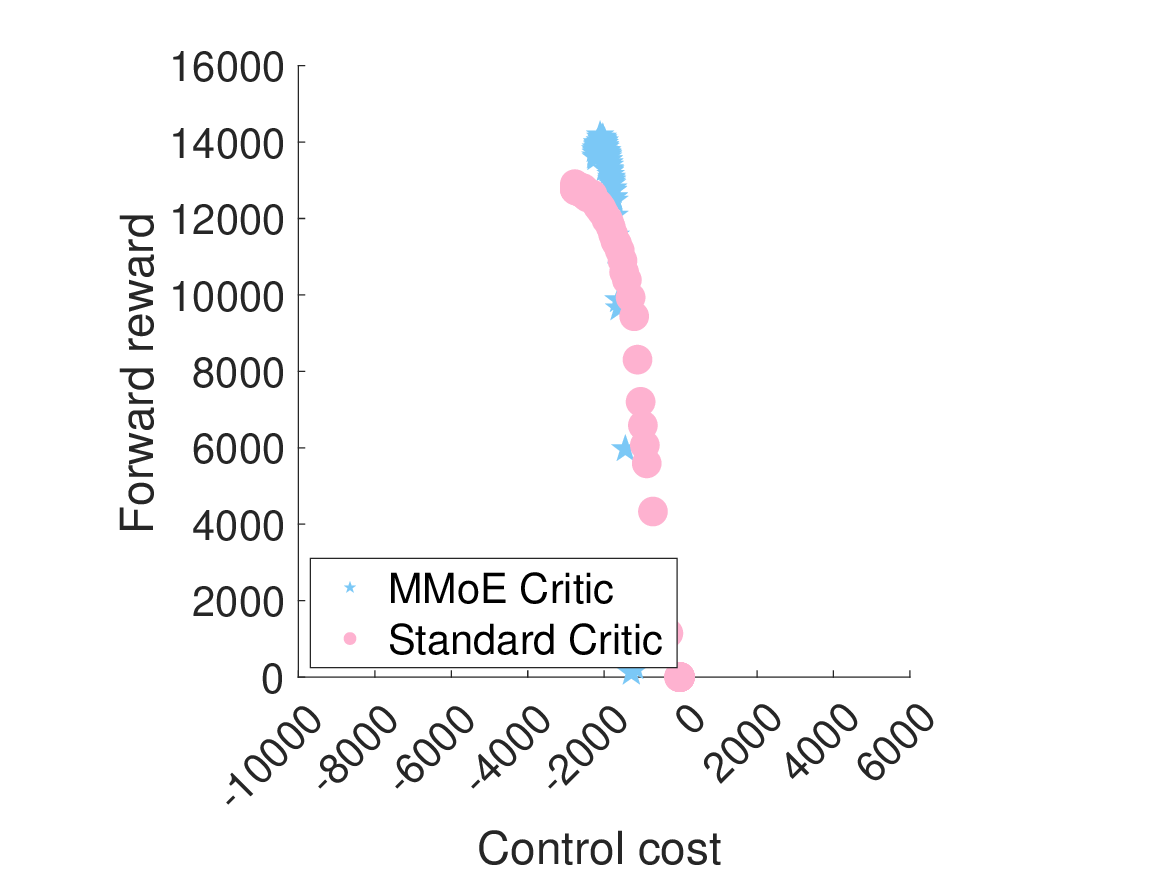}} 
    \label{fig:MMOEhv_hc}

    &\hspace{-5mm} \scalebox{0.5}{\includegraphics[width=\textwidth]{./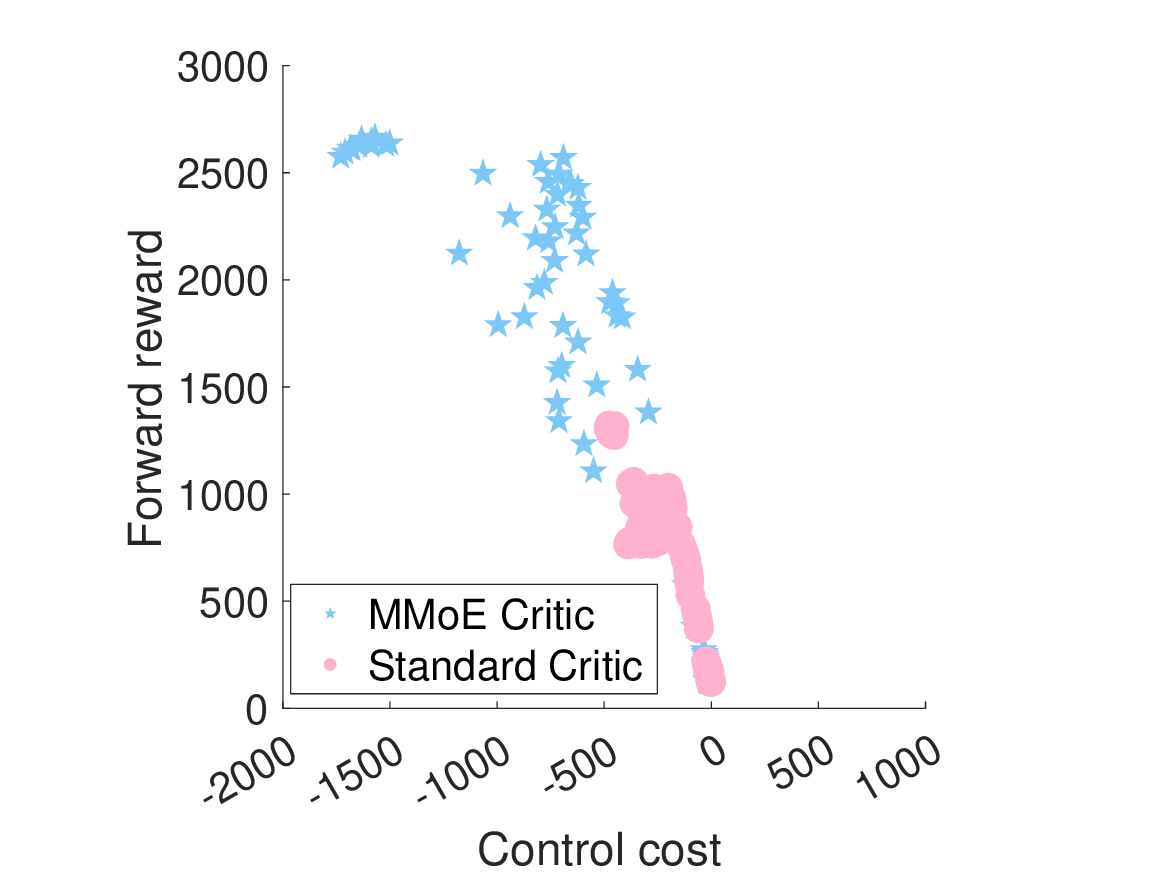}}  
    \label{fig:MMOEhv_hopper}\\
    \mbox{\hspace{-0mm}\small (a) HalfCheetah} & \hspace{-2mm} \mbox{\small (b) Hopper}  \\
\end{array}$
\caption{Solution set of MOSAC with MMoE structure critic and Standard structure}
\label{fig:MMOEHV}
\end{figure*}

\begin{figure*}[!tb]
\centering
$\begin{array}{c c c}
    \multicolumn{1}{l}{\mbox{\bf }} & \multicolumn{1}{l}{\mbox{\bf }} \\ 
    \hspace{-0mm} \scalebox{0.5}{\includegraphics[width=\textwidth]{./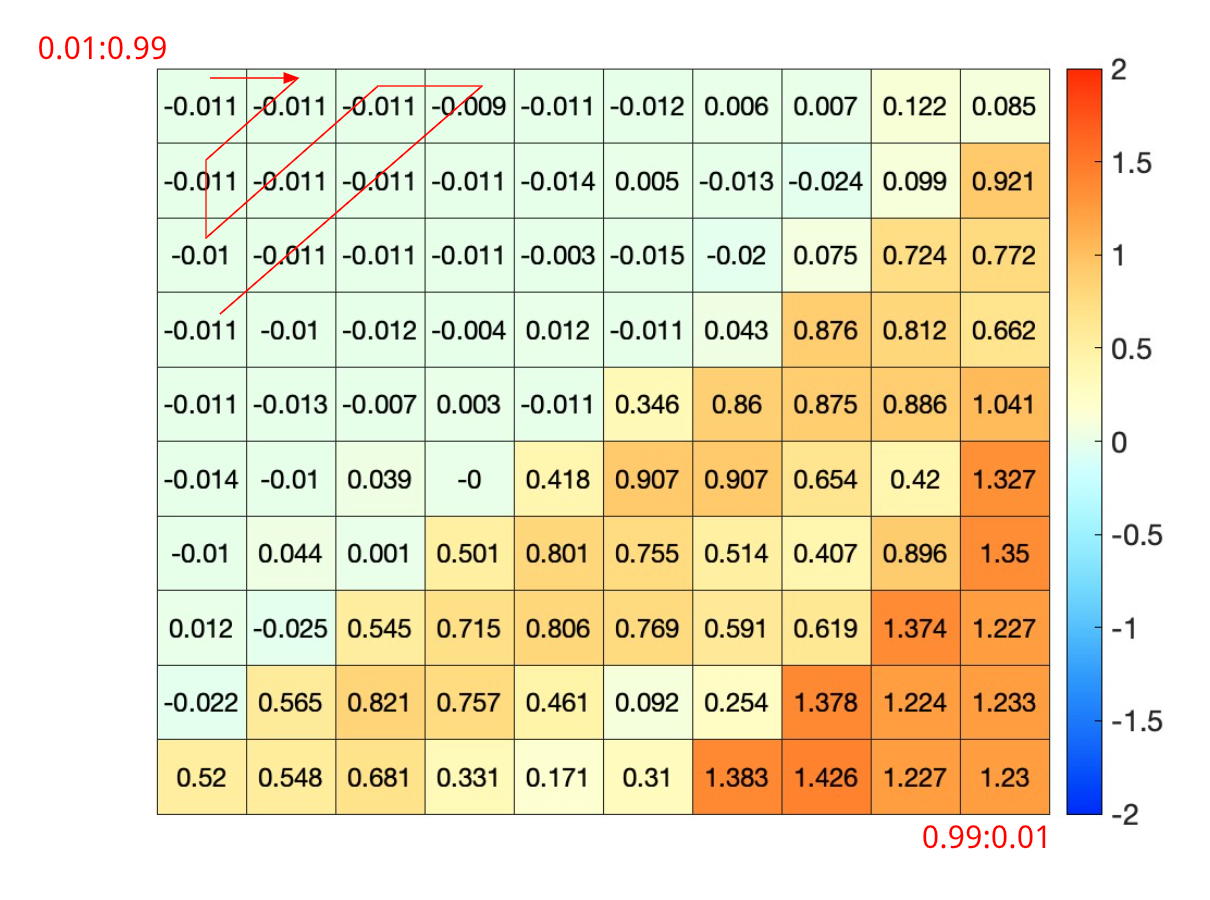}} 
    \label{fig:EPD_hc}

    &\hspace{5mm} \scalebox{0.5}{\includegraphics[width=\textwidth]{./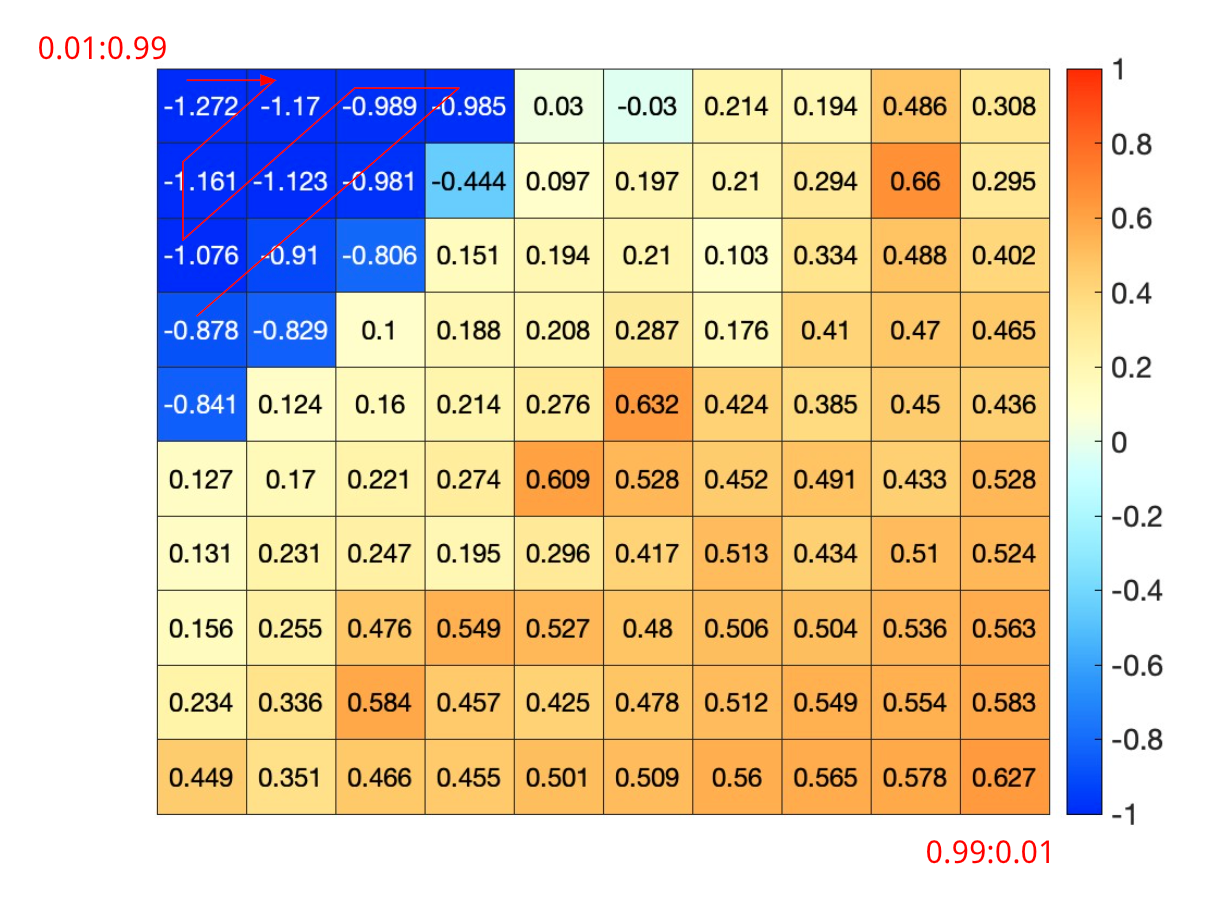}}  
    \label{fig:EPD_hopper}\\
    \mbox{\hspace{-0mm}\small (a) HalfCheetah} & \hspace{-2mm} \mbox{\small (b) Hopper}  \\
\end{array}$
\caption{100 preferences total reward comparing of MMoE structure critic and standard structure for 1 seed. We set MMoE total reward to $\mathcal{M}$, Standard total reward to $\mathcal{S}$ and the value in cell is $ (\mathcal{M}-\mathcal{S})/1000 $ and we plot the 100 preferences with zig-zag way.}
\label{fig:MMOEEPD}
\end{figure*}

\begin{minipage}{\textwidth}
  \begin{minipage}[t]{0.3\textwidth} %trying to force figs apart
    \includegraphics[width=\linewidth]{./images/reward91_monovsdual.eps}
  \end{minipage}%
  \begin{minipage}[t]{0.3\textwidth} %trying to force figs apart
    \includegraphics[width=\linewidth]{./images/reward91_monovsdual.eps}
  \end{minipage}%
  \hfill
  \begin{minipage}[b]{0.49\textwidth}
    \centering
    \label{tab:MMOE result}
    \begin{tabular}{l c c c }
         \hline Environments & Metrics & \textbf{Standard} & \textbf{MMoE} \\
         \hline
         \hline
          & HV($\times 10^7$) & \textbf{3.3} & 3.1\\
         \cline{2-4}
         HalfCheetah & UT($\times 10^3$) &  5.0& \textbf{5.5}\\
         \cline{2-4}
          & EPD &   - &  \textbf{0.74}\\
         \hline
          & HV($\times 10^6$)& 1.1 & \textbf{1.5}\\
         \cline{2-4}
         Hopper & UT($\times 10^2$) & 4.2 & \textbf{5.6} \\
         \cline{2-4}
          & EPD &  - & \textbf{0.64}\\
         
         \hline
    \end{tabular}
      \captionof{table}{A table beside a figure}
    \end{minipage}
  \end{minipage}
  
  \begin{table*}[!htb]
    \centering
    \caption{Comparison with MMoE critic and Normal critic using three metric. The ED is calculated by comparing to Standard MOSAC. And we use different reference point from Table \ref{tab:expResult} to calculate in hopper due to the larger control cost.}
    \label{tab:MMOE result}
    \begin{tabular}{l c c c }
         \hline Environments & Metrics & \textbf{Standard MOSAC} & \textbf{MMoE MOSAC} \\
         \hline
         \hline
          & HV($\times 10^6$) & \textbf{33.05} & 30.87\\
         \cline{2-4}
         HalfCheetah & UT &  4973.31& \textbf{5463.10}\\
         \cline{2-4}
          & ED &   - &  \textbf{0.74}\\
         \hline
          & HV($\times 10^5$)& 2.12 & \textbf{2.53}\\
         \cline{2-4}
         Hopper & UT & 301.58 & \textbf{561.32} \\
         \cline{2-4}
          & ED &  - & \textbf{0.64}\\
         
         \hline
    \end{tabular}
\end{table*}

\begin{figure*}[!htb]
\centering
$\begin{array}{c c c}
    \multicolumn{1}{l}{\mbox{\bf }} & \multicolumn{1}{l}{\mbox{\bf }} \\ 
    \hspace{-0mm} \scalebox{0.5}{\includegraphics[width=\textwidth]{./images/MMOEhv_half_cheetah.eps}} 
    \label{fig:MMOEhv_hc}

    &\hspace{-5mm} \scalebox{0.5}{\includegraphics[width=\textwidth]{./images/MMOEhvhopper.eps}}  
    \label{fig:MMOEhv_hopper}\\
    \mbox{\hspace{-0mm}\small (a) HalfCheetah} & \hspace{-2mm} \mbox{\small (b) Hopper}  \\
\end{array}$
\caption{Solution set of MOSAC with MMoE structure critic and Standard structure}
\label{fig:MMOEHV}
\end{figure*}
