# Supplementary material for: Q-Pensieve: Boosting Sample Efficiency of Multi-Objective RL Through Memory Sharing of Q-Snapshots
Source: arXiv:2212.03117 source file (2024-07-25)
Supplement: Supplementary file 2 [file 8-Appendix.tex]

\newpage
\appendix
\section{Appendix}
\label{section:Appendix}
\subsection{Proofs}

% \label{lemma:Soft policy evaluation}
% Since we learn a set of policies for different preference simultaneously
% Consider the soft Bellman backup operator $\mathcal{T}^{\pi}$ and define $Q_{k+1} =\mathcal{T}^{\pi}Q_k$. Then $Q_k$ will converge to the soft Q-value of $\pi$ as $k \rightarrow \infty$.
% \begin{align}
%     (\cT^{\pi}Q_{k})(s,a;\omega)=r(s,a)+\gamma\E_{s'\sim P(\cdot|s,a),a'\sim\pi(\cdot|s')}[Q_{k}(s',a';\omega)-\alpha 1_d \log \pi(a'|s')],\label{eq:Lemma_eva_line1}\\
%     Q_{k+1}(s_{k+1},a_{k+1};\omega) \leftarrow r(s_{k},a_{k})+\gamma\E_{s_{k}\sim P,a_{k}\sim\pi}[Q_{k}(s_{k},a_{k};\omega)-\alpha 1_d\log \pi(a_{k}|s_{k})].\label{eq:Lemma_eva_line2}
% \end{align}
% where (\ref{eq:Lemma_eva_line1}) is a direct result of (\ref{eq:Lemma_eva_line2}) followed from $Q_{k+1} =\mathcal{T}^{\pi}Q_k$. \\
\begin{myproof}[Lemma \ref{lemma:Soft policy evaluation}]
\normalfont  
Define the entropy augmented reward as $
r_{\pi}(s,a)=r(s,a)-\gamma\E_{s\sim P,a\sim\pi}[\alpha 1_d\log \pi(a|s)]$, and rewrite the update rule as
\begin{equation}
Q(s,a;\omega)\leftarrow r_{\pi}(s,a)+\gamma\E_{s'\sim P,a'\sim\pi}[Q(s',a';\omega)]
\label{eq:Lemma_eva_line2}.
\end{equation}
Apply the standard convergence result for policy evaluation.(\cite{Sutton1998}), the entropy augmented reward is bounded.

\end{myproof}

% \label{lemma:Soft Policy Improvement}
% Let $\pi_{old}\in\Pi$ and let $\pi_{new}$ be the optimizer of the minimization problem defined in (\ref{eq:pinew equality})
% . Then $Q^{\pi_{new}} (s_t, a_t) \leq Q^{\pi_{old}} (s_t, a_t)$ for all $(s_t, a_t) \in \cS \times \cA$ with $|\cA| < \infty$\\
\begin{myproof}[Lemma \ref{lemma:Soft Policy Improvement}]
\normalfont
Let $\pi_{old}\in\Pi$ with parameter $\phi_{old}$ and let $Q^{\pi_{old}}$ and $V^{\pi_{old}}$ be the corresponding soft state-action value and soft state value, and let $\pi_{new}$ be defined as 
\begin{align}
\pi_{new}&=\arg\min_{\pi'\in\Pi}D_{KL}(\pi'(\cdot|s';\omega)||\exp(\sup_{\omega'\in\Omega,Q \in \cQ}\omega^\intercal Q(s,\cdot;\omega')-\log Z_{\mathcal{Q}}(s_t)))\label{eq:pinew equality 1}\\
&=\arg\min_{\pi'\in\Pi}J_{\pi_{old}}(\phi_{old};\omega)\label{eq:pinew equality 2}.
\end{align}

Since $J_{\pi_{old}}(\phi_{old};\omega)\leq J_{\pi_{old}} (\phi_{new};\omega)$, we have 

\begin{align}
\E_{a_t\sim\pi_{new}}[\alpha \cdot 1_d\log \pi_{new}(a_t|s_t)-\sup_{\omega'\in\Omega, Q \in \cQ}\omega^\intercal Q(s_t,a_t;\omega)+\log Z_{\mathcal{Q}}(s_t)] \nonumber\\ \leq \E_{a_t\sim\pi_{old}}[\alpha \cdot 1_d\log \pi_{old}(a_t|s_t)-\sup_{\omega'\in\Omega,Q \in \cQ}\omega^\intercal Q(s_t,a_t;\omega)+\log Z_{\mathcal{Q}}(s_t)],
\end{align} 
and due to $Z_{\mathcal{Q}}$ only depends on the state, the inequality reduces to \begin{align}
&\E_{a\sim\pi_{new}}[\alpha \cdot 1_d log\pi_{new}(\cdot|s) - \sup_{\omega'\in\Omega,Q \in \cQ}\omega^\intercal Q^{\pi_{old}}(s,a;\omega)]\nonumber
\\&\leq\E_{a\sim\pi_{old}}[\alpha \cdot 1_d log\pi_{old}(\cdot|s) - \sup_{\omega'\in\Omega,Q \in \cQ}\omega^\intercal Q^{\pi_{old}}(s,a;\omega)]\label{Soft Policy Improvement:equ1}
\\&\E_{a\sim\pi_{old}}[\sup_{\omega'\in\Omega,Q \in \cQ }\omega^\intercal Q^{\pi_{old}}(s,a;\omega) - \alpha \cdot 1_d log\pi_{old}(\cdot|s)]\nonumber
\\&\leq \E_{a\sim\pi_{new}}[-\alpha \cdot 1_d log\pi_{new}(\cdot|s)]+\E_{a'\sim\pi_{new}}[\sup_{\omega'\in\Omega,Q \in \cQ}\omega^\intercal Q(s,a';\omega)]\label{Soft Policy Improvement:equ2}
\end{align}
where (\ref{Soft Policy Improvement:equ2}) is direct result of (\ref{Soft Policy Improvement:equ1}).\\
Next, consider the soft Bellman equation:
\begin{align}
\omega^\intercal Q^{\pi_{old}}(s,a;\omega)& =\omega^\intercal r(s,a)+\gamma\omega^\intercal \E_{s'\sim P(\cdot|(s,a)),a'\sim \pi_{old}(\cdot|s')}[Q^{\pi_{old}}(s',a';\omega)-\alpha\cdot 1_d\log(\pi_{old}(\cdot|s'))] \label{Soft Policy Improvement:equ3}
\\&\leq\omega^\intercal r(s,a)+\gamma\omega^\intercal \E_{s'\sim P(\cdot|(s,a))}[-\E_{a'\sim \pi_{new}(\cdot|s')}[\alpha\cdot 1_d\log(\pi_{old}(\cdot|s'))]\nonumber
\\&+\E_{a'\sim \pi_{new}(\cdot|s')}[\sup_{\omega'\in\Omega,Q \in \cQ}\omega^\top Q(s',a';\omega')]] \label{Soft Policy Improvement:equ4}
\\&\leq\omega^\intercal r(s,a)-\gamma\E_{s'\sim P(\cdot|(s,a)),a'\sim \pi_{new}(\cdot|s')}[\alpha\cdot 1_d\log(\pi_{new}(\cdot|s'))]\nonumber
\\&+\gamma\E_{s'\sim P(\cdot|(s,a)),a'\sim \pi_{old}(\cdot|s')}[\omega^\intercal r(s',a')]\nonumber
\\&-\gamma^2\E_{s''\sim P(\cdot|(s',a')),a''\sim \pi_{new}(\cdot|s'')}[\alpha\cdot 1_d\log(\pi_{new}(\cdot|s''))]\nonumber
\\&+\gamma^2\E_{s''\sim P(\cdot|(s',a')),a''\sim \pi_{old}(\cdot|s'')}[\omega^\intercal r(s'',a'')]\cdots \label{Soft Policy Improvement:equ5}
\\&=\omega^\intercal r(s,a))-\gamma\E_{s'\sim P(\cdot|(s,a)),a'\sim \pi_{new}(\cdot|s')}[\alpha\cdot 1_d\log(\pi_{new}(\cdot|s'))]\nonumber
\\&+\gamma\omega^\intercal r(s',a'))-\gamma^2\E_{s''\sim P(\cdot|(s',a')),a''\sim \pi_{new}(\cdot|s'')}[\alpha\cdot 1_d\log(\pi_{new}(\cdot|s''))]\cdots \label{Soft Policy Improvement:equ6}
\\&=R(s,a)+\gamma R(s',a')+\gamma^2R(s'',a'')\cdots \label{Soft Policy Improvement:equ7}
\\&=\omega^\intercal Q^{\pi_{new}}(s,a;\omega), \label{Soft Policy Improvement:equ8}
\end{align}
where (\ref{Soft Policy Improvement:equ3}) is adjusted from (\ref{eq:Lemma_eva_line2}), (\ref{Soft Policy Improvement:equ4}) is hold by (\ref{Soft Policy Improvement:equ2}). (\ref{Soft Policy Improvement:equ5}), (\ref{Soft Policy Improvement:equ6}) is reduced from (\ref{Soft Policy Improvement:equ4}). And then we define $R(s,a)$ as $\omega^\intercal r(s,a)-\gamma\E_{s'\sim P(\cdot|(s,a)),a'\sim \pi_{new}(\cdot|s')}[\alpha\cdot 1_d\log(\pi_{new}(\cdot|s'))]$, so we can rewrite (\ref{Soft Policy Improvement:equ6}) as (\ref{Soft Policy Improvement:equ7}). Due to the definition of $Q$-function, we can replace the result with (\ref{Soft Policy Improvement:equ8}), and then we get $\sup_{\omega'\in\Omega Q \in \cQ}\omega^\intercal Q^{\pi_{old}}(s,a;\omega) \leq \sup_{\omega'\in\Omega Q \in \cQ}\omega^\intercal Q^{\pi_{new}}(s,a;\omega)$. Convergence to $Q^{\pi_{new}}$ follows from Lemma \ref{lemma:Soft policy evaluation}.
\end{myproof}

\subsection{Training Details}
We conduct all experiment on baselines with following hyper parameters.
\begin{table}[]
\centering
\caption{MOSAC Hyperparameters}
\label{tab:MOSAC_hyperparameters}
\begin{tabular}{ll}
Parameter                        & Value   \\ \hline
optimizer                        & Adam    \\
learning rate                    & 0.0003  \\
discount                         & 0.99    \\
replay buffer size               & 1000000 \\
depth of hidden layers           & 2       \\
number of hidden units per layer & 256     \\
number of samples per minibatch  & 256     \\
nonlinearity                     & ReLU    \\
target smoothing coefficient     & 0.005   \\
target update interval           & 1       \\
gradient steps                   & 1      
\end{tabular}
\end{table}

\subsection{Experiments Details}

\subsubsection{Learning curve comparison}
We demonstrate the learning curve for different baselines, and SAC would be trained in the fixed preference. We can find that MOSAC nearly behaves as well as SAC does in some situations and beats other baselines.

\begin{figure*}[!tb]
\centering
$\begin{array}{c c c}
    \multicolumn{1}{l}{\mbox{\bf }} & \multicolumn{1}{l}{\mbox{\bf }} & \multicolumn{1}{l}{\mbox{\bf }} \\ 
    \hspace{-0mm} \scalebox{0.33}{\includegraphics[width=\textwidth]{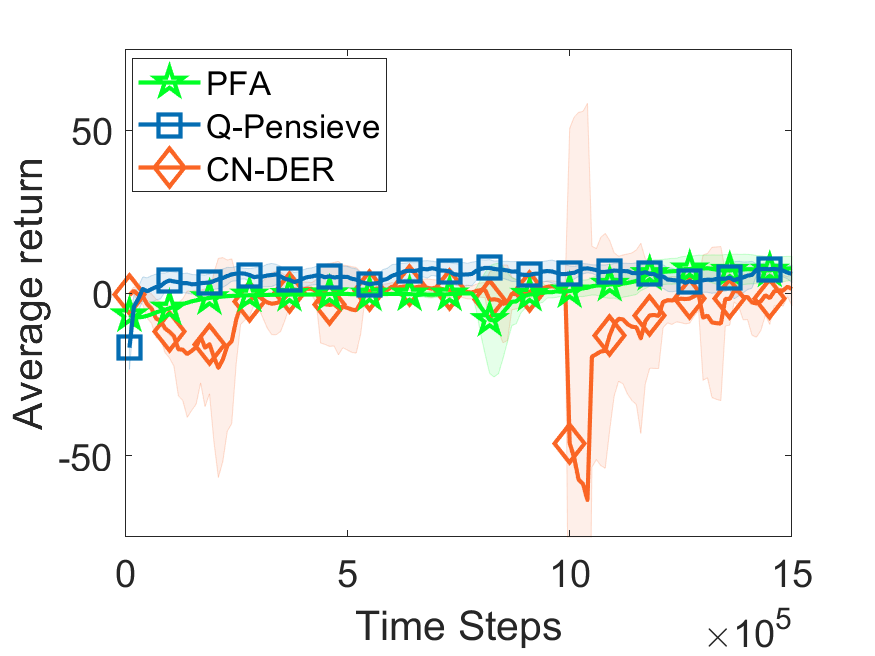}} \label{fig:hopper_learning_curve19}
    & \hspace{-5mm} \scalebox{0.33}{\includegraphics[width=\textwidth]{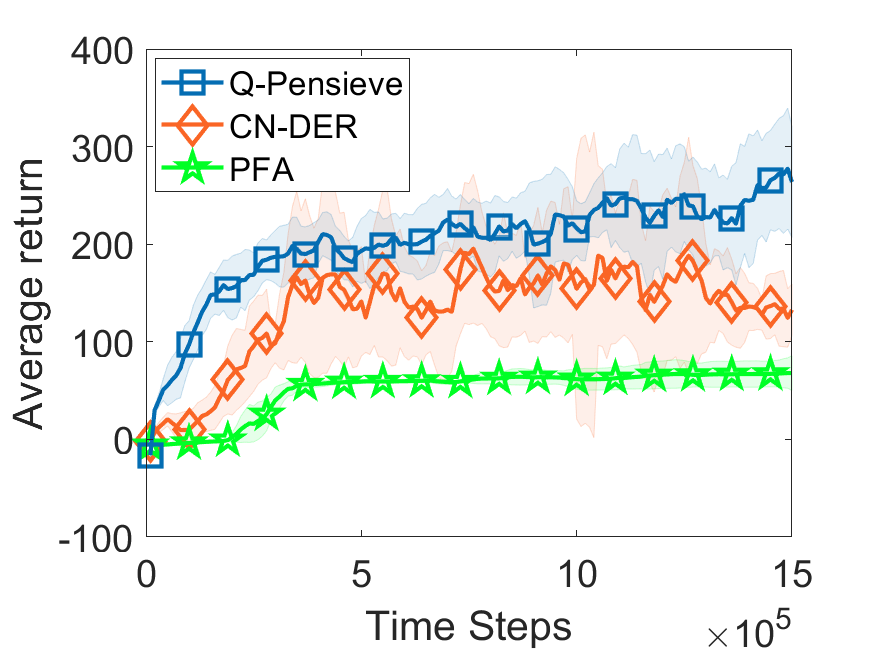}} \label{fig:hopper_learning_curve55}
    &\hspace{-5mm} \scalebox{0.33}{\includegraphics[width=\textwidth]{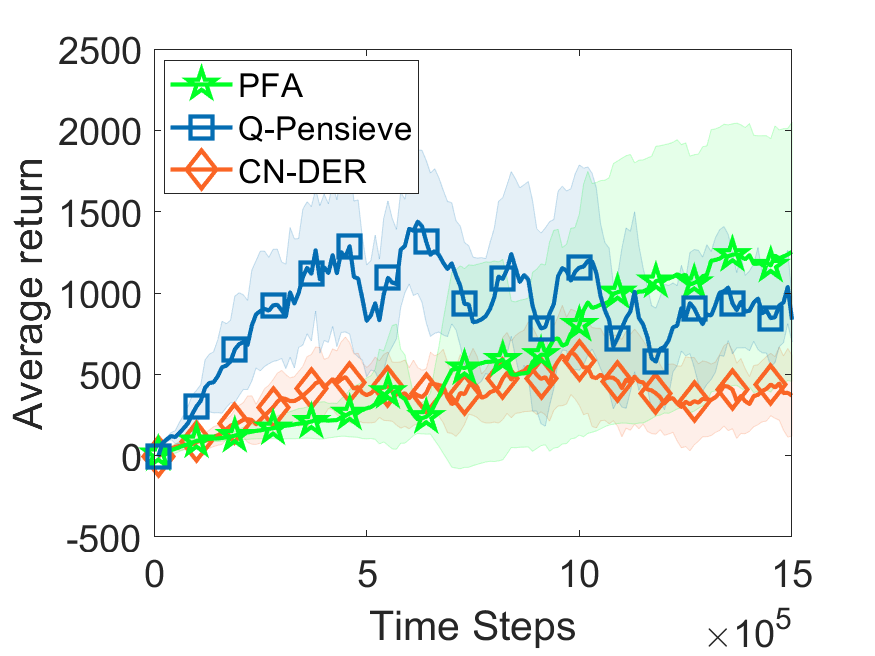}}  \label{fig:hopper_learning_curve91}\\
    \mbox{\hspace{-0mm}\small (a)$\omega = [0.1, 0.9]$} & \hspace{-2mm} \mbox{\small (b)$\omega = [0.5, 0.5]$} & \hspace{-2mm} \mbox{\small (c)$\omega = [0.9, 0.1]$} \\
\end{array}$
\caption{Average return over 5 random seeds in Hopper: Average return is inner product of distinct reward vectors and the corresponding preference.}
\label{fig:hopper_learning_curve}
\end{figure*}

\begin{figure*}[!tb]
\centering
$\begin{array}{c c c}
    \multicolumn{1}{l}{\mbox{\bf }} & \multicolumn{1}{l}{\mbox{\bf }} & \multicolumn{1}{l}{\mbox{\bf }} \\ 
    \hspace{-0mm} \scalebox{0.33}{\includegraphics[width=\textwidth]{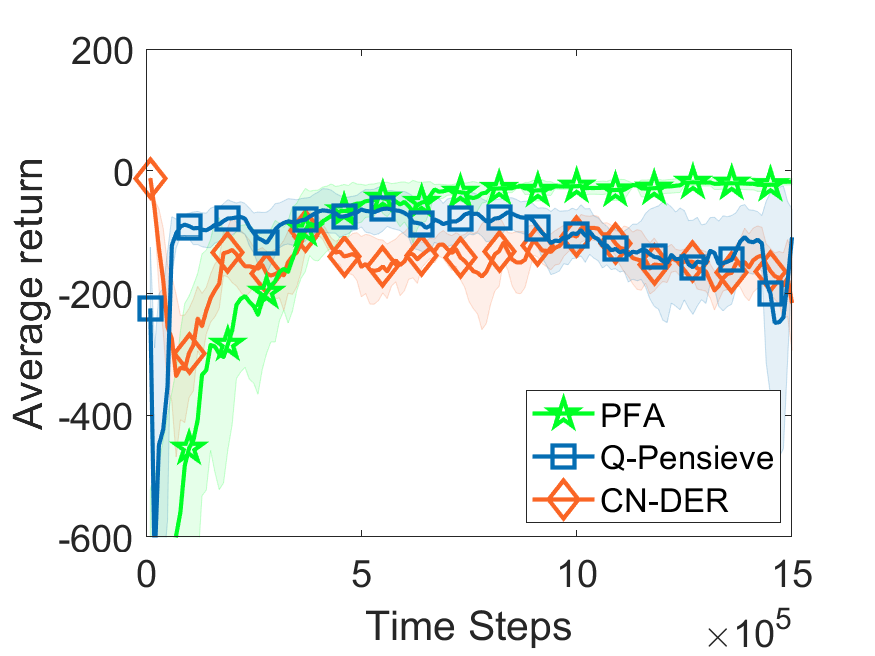}} \label{fig:ant_learning_curve19}
    & \hspace{-5mm} \scalebox{0.33}{\includegraphics[width=\textwidth]{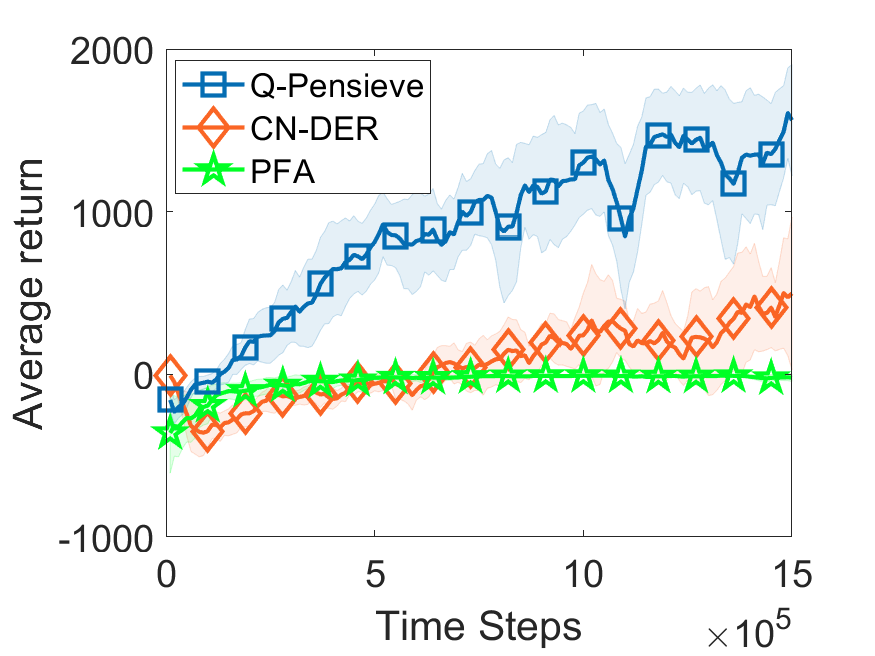}} \label{fig:ant_learning_curve55}
    &\hspace{-5mm} \scalebox{0.33}{\includegraphics[width=\textwidth]{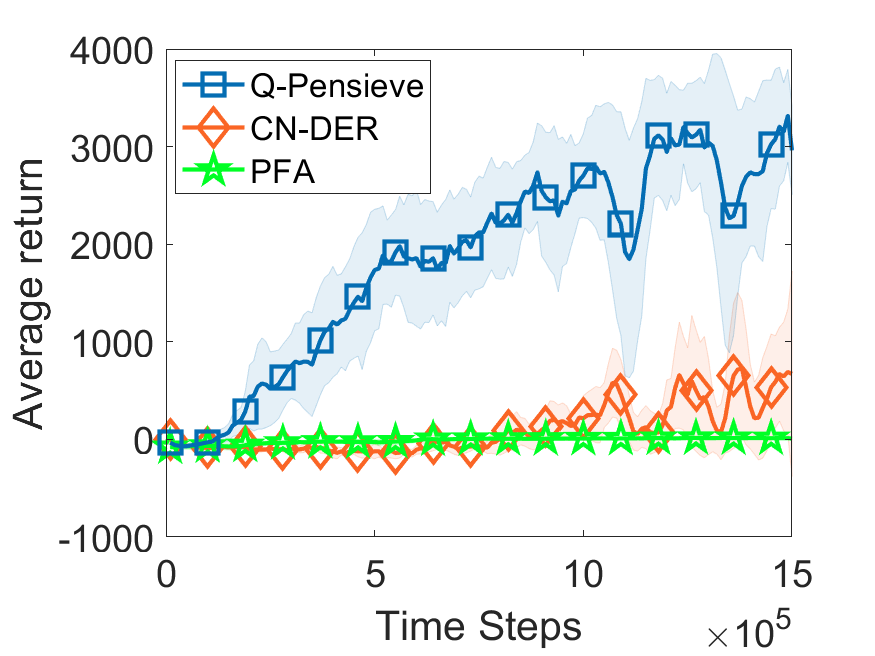}}  \label{fig:ant_learning_curve91}\\
    \mbox{\hspace{-0mm}\small (a)$\omega = [0.1, 0.9]$} & \hspace{-2mm} \mbox{\small (b)$\omega = [0.5, 0.5]$} & \hspace{-2mm} \mbox{\small (c)$\omega = [0.9, 0.1]$} \\
\end{array}$
\caption{Average return in Ant over 5 random seeds : Average return is inner product of distinct reward vectors and the corresponding preference.}
\label{fig:ant_learning_curve}
\end{figure*}
\begin{figure*}[!tb]
\centering
$\begin{array}{c c c}
    \multicolumn{1}{l}{\mbox{\bf }} & \multicolumn{1}{l}{\mbox{\bf }} & \multicolumn{1}{l}{\mbox{\bf }} \\ 
    \hspace{-0mm} \scalebox{0.33}{\includegraphics[width=\textwidth]{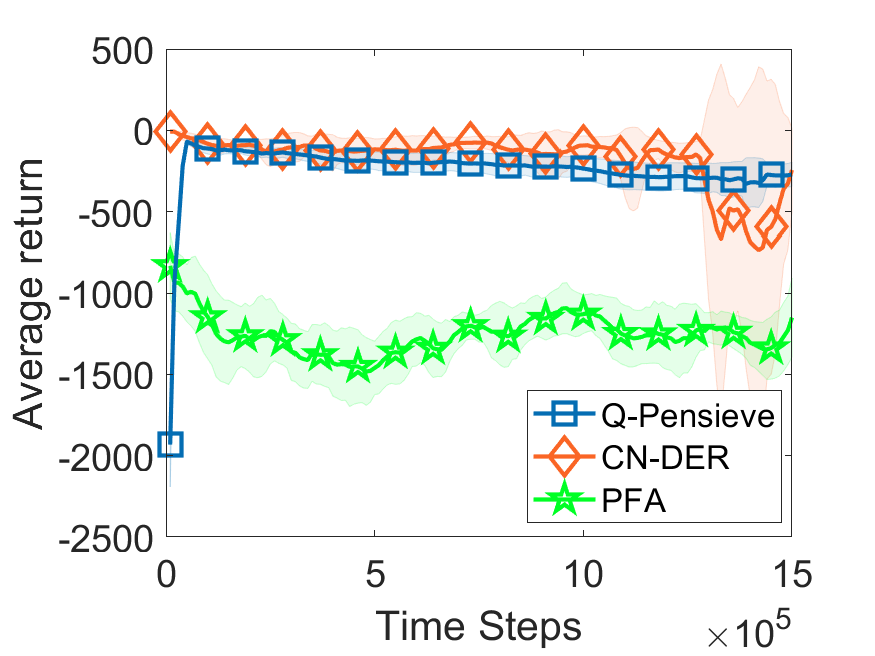}} \label{fig:half_cheetah_learning_curve19}
    & \hspace{-5mm} \scalebox{0.33}{\includegraphics[width=\textwidth]{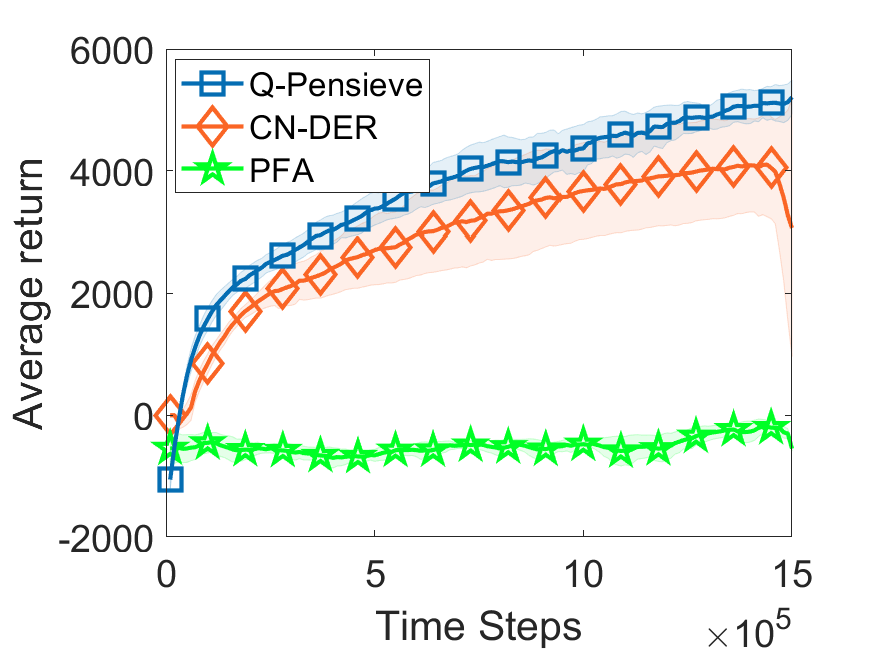}} \label{fig:half_cheetah_learning_curve55}
    &\hspace{-5mm} \scalebox{0.33}{\includegraphics[width=\textwidth]{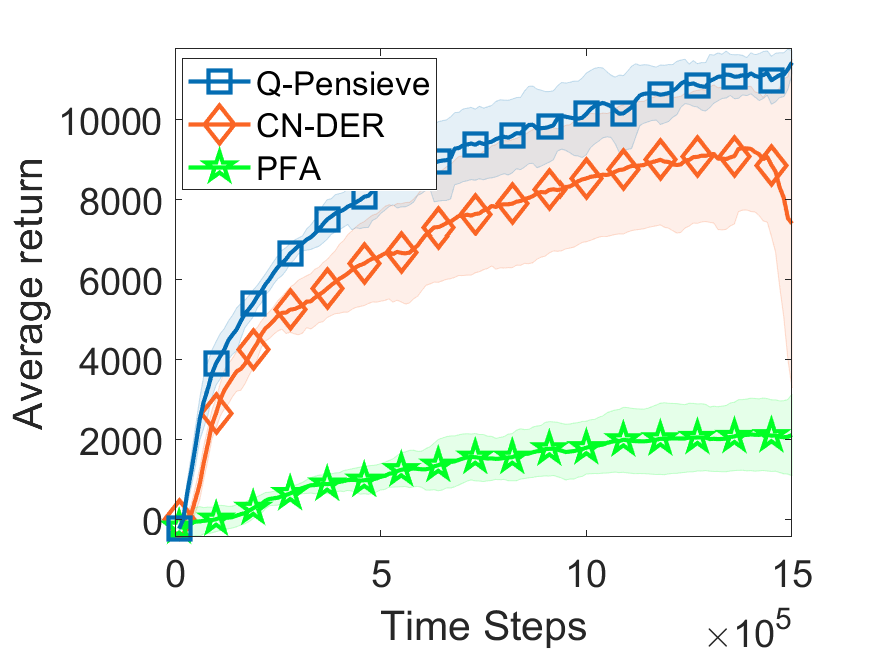}}  \label{fig:half_cheetah_learning_curve91}\\
    \mbox{\hspace{-0mm}\small (a)$\omega = [0.1, 0.9]$} & \hspace{-2mm} \mbox{\small (b)$\omega = [0.5, 0.5]$} & \hspace{-2mm} \mbox{\small (c)$\omega = [0.9, 0.1]$} \\
\end{array}$
\caption{Average return in over 5 random seeds  HalfCheetah: Average return is inner product of distinct reward vectors and the corresponding preference.}
\label{fig:half_cheetah_learning_curve}
\end{figure*}
\begin{figure*}[!tb]
\centering
$\begin{array}{c c c}
    \multicolumn{1}{l}{\mbox{\bf }} & \multicolumn{1}{l}{\mbox{\bf }} & \multicolumn{1}{l}{\mbox{\bf }} \\ 
    \hspace{-0mm} \scalebox{0.33}{\includegraphics[width=\textwidth]{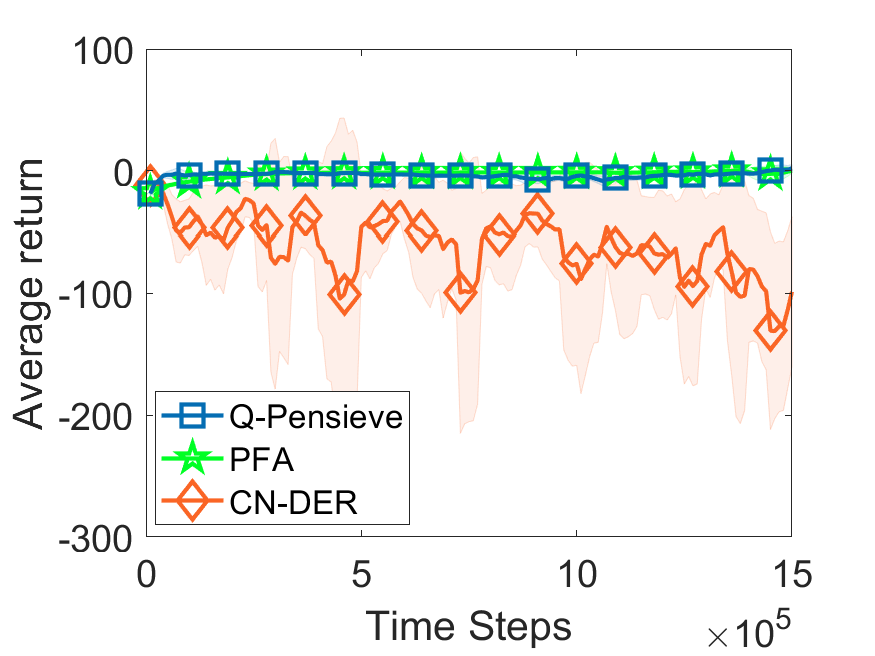}} \label{fig:walker_learning_curve19}
    & \hspace{-5mm} \scalebox{0.33}{\includegraphics[width=\textwidth]{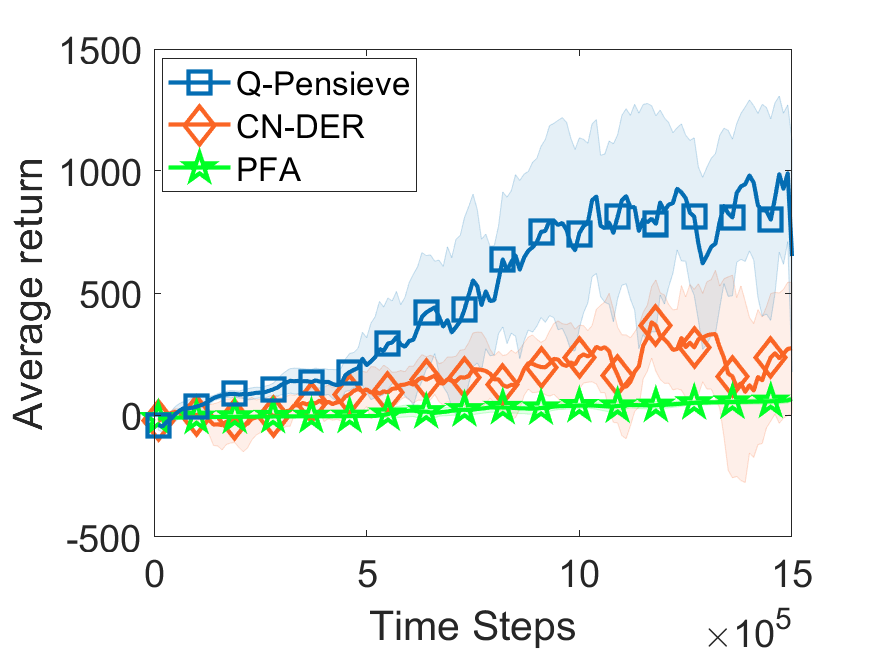}} \label{fig:walker_learning_curve55}
    &\hspace{-5mm} \scalebox{0.33}{\includegraphics[width=\textwidth]{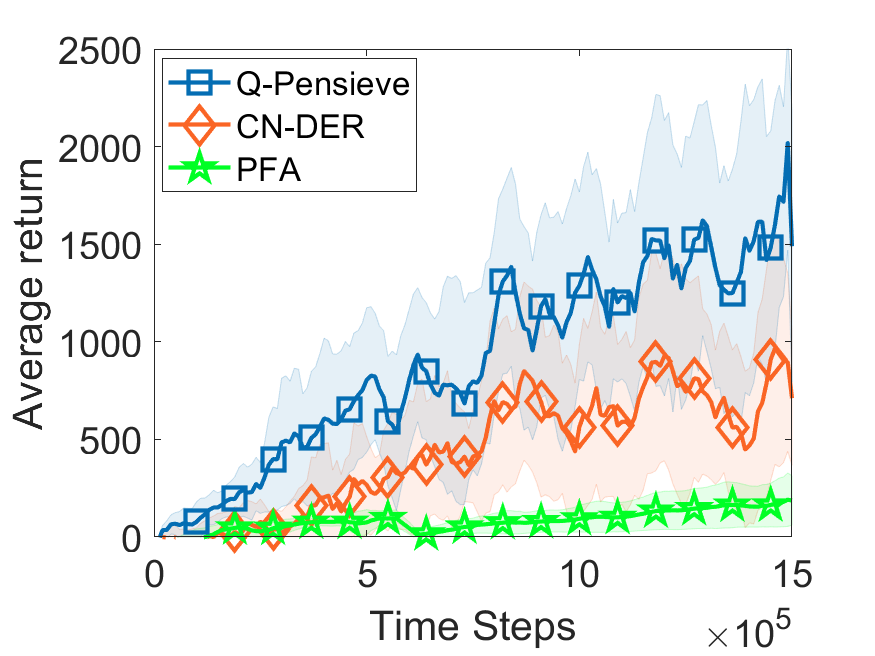}}  \label{fig:walker_learning_curve91}\\
    \mbox{\hspace{-0mm}\small (a)$\omega = [0.1, 0.9]$} & \hspace{-2mm} \mbox{\small (b)$\omega = [0.5, 0.5]$} & \hspace{-2mm} \mbox{\small (c)$\omega = [0.9, 0.1]$} \\
\end{array}$
\caption{Average return in Walker2d over 5 random seeds : Average return is inner product of distinct reward vectors and the corresponding preference.}
\label{fig:walker_learning_curve}
\end{figure*}
